# Supplementary material for: Enumerating meandric systems with large number of loops
Source: arXiv:1609.02756 ancillary file (2017-07-10)
Supplement: Supplementary file 1 [file irred-power-series-ab.pdf]

```

In[1097]:= ClearAll["Global`*"];

In[1176]:= CompatibleRAB[r_, a_, b_] := Module[{},
  If[Abs[a - b] > r, Return[False]];
  If[a + b < r, Return[False]];
  If[a > 2 * r - 2 && r ≥ 2, Return[False]];
  If[b > 2 * r - 2 && r ≥ 2, Return[False]];
  If[Mod[Abs[a - b] - r, 2] ≠ 0, Return[False]];
  If[r == Abs[a - b] && Min[a, b] > 0, Return[False]];
  Return[True];
];

IFromFile[r_, a_, b_, verbose_: False] :=
Module[{f, i, j, k, filename, q, n, p, plist},
  (* Computes, from the text filex containing the
    number of irreducible meanders, the I series *)
  f = 0;
  SetDirectory[NotebookDirectory[]];
  For[k = 0, k ≤ r, k++,
    For[i = 0, i ≤ a, i++,
      For[j = i, j ≤ b, j++,
        filename =
          StringForm["irred-``-``-``.txt", k, Min[i, j], Max[i, j]] // ToString;
        If[verbose, Print["Filename: ", filename]];
        If[FileExistsQ[filename],
          plist = Get[filename];
          If[verbose, Print["Data: ", plist]];
          For[q = 1, q ≤ Length[plist], q++,
            p = plist[[q, 1]];
            n = plist[[q, 2]];
            f += n * X^p * Y^k * A^i * B^j;
            If[i < j, f += n * X^p * Y^k * A^j * B^i];
          ];];];];
  Simplify[f]
];

MomentCumulantXYAB[f_, rmax_, amax_, bmax_, prefix_, verbose_: False] := Module[
  {g, r, a, b, filename, eqs, curSol, sc, css, ff, goodSol, i, gg, rr, aa, bb},
  SetDirectory[NotebookDirectory[]];
  g = 0;
  For[r = 0, r ≤ rmax, r++,
    For[a = 0, a ≤ amax, a++,
      For[b = 0, b ≤ bmax, b++,
        If[CompatibleRAB[r, a, b],
          g = g + c[Min[a, b], Max[a, b], r] * A^a * B^b * Y^r;
        ]];];
  If[verbose, Print["g=", g]];
  For[r = 0, r ≤ rmax, r++,
    For[a = 0, a ≤ amax, a++,
      For[b = a, b ≤ bmax, b++,
        If[CompatibleRAB[r, a, b],
          If[verbose,
            Print["Compatible triple found --- r=", r, " a=", a, " b=", b]];
          filename = StringForm[prefix <> "-``-``-``.txt", r,
            Min[a, b], Max[a, b]] // ToString;
          If[verbose, Print["Trying to read from file ", filename]];
          If[FileExistsQ[filename],
            (* the coefficient was computed, get if from the file *)
            If[verbose, Print["File exists, reading solution"]];
            curSol = Get[filename];
            (* Updating g *)

```

```

g = g /. curSol;
If[b > a,
  css = curSol /. {c[a, b, r] → c[b, a, r]};
  g = g /. css;
];
,
(* if the coefficient was not computed, do it now *)
If[verbose, Print["File does not exist, computing solution"]];
(* preparing the equation to solve for the current coefficient *)
gg = g;
For[rr = 0, rr ≤ rmax, rr++,
  For[aa = 0, aa ≤ amax, aa++,
    For[bb = aa, bb ≤ bmax, bb++,
      If[rr > r || (rr == r && aa > a) || (rr == r && aa == a && bb > b),
        gg = gg /. {c[aa, bb, rr] → 0}];
    ]];
If[verbose, Print["Begin... Expand with gg=", gg]];
ff = f /. {X → X + X*gg};
If[verbose, Print["end Expand"]];
eqs = ff - gg;
(*If[verbose, Print["eqs=", eqs]];*)
sc = SeriesCoefficient[eqs, {Y, 0, r}, {B, 0, b}, {A, 0, a}];
If[verbose, Print["sc=", sc]];
If[verbose,
  Print["Coefficient r=", r, " a=", a, " b=", b, " computed."]];
curSol = Solve[0 == sc, c[a, b, r]];
If[verbose, Print["solutions found: ", curSol]];
(* we need to find the right solution -
  this is the one starting with W *)
goodSol = 0;
For[i = 1, i ≤ Length[curSol], i++,
  If[Limit[(c[a, b, r] /. curSol[[i]]), X → 0] == 0, goodSol = i]];
If[verbose, Print["Equation solved, correct solution is ", goodSol]];
curSol = FullSimplify[curSol[[goodSol]], X > 0 && X < 1/4];
(* write the coefficient in the file *)
Put[curSol, filename];
];
If[verbose, Print["We have solution: ", curSol]];
g = g /. curSol;
If[b > a,
  css = curSol /. {c[a, b, r] → c[b, a, r]};
  If[verbose, Print[css]];
  g = g /. css;
];
If[verbose, Print["End stuff"]];
]]];
Collect[g, {Y, A, B}]
];
MomentCumulantWYAB[f_, rmax_, amax_, bmax_, prefix_, verbose_: False] :=
Module[{g, r, a, b, filename, eqs, curSol, sc,
  css, ff, goodSol, i, j, k, toExpand, gg, rr, aa, bb},
  SetDirectory[NotebookDirectory[]];
  g = 0;
  For[r = 0, r ≤ rmax, r++,
    For[a = 0, a ≤ amax, a++,
      For[b = 0, b ≤ bmax, b++,
        If[CompatibleRAB[r, a, b],
          g = g + c[Min[a, b], Max[a, b], r] * A^a * B^b * Y^r;
        ]];
  ]];

```

```

If[verbose, Print["g=", g]];
For[r = 0, r ≤ rmax, r++,
  For[a = 0, a ≤ amax, a++,
    For[b = a, b ≤ bmax, b++,
      If[CompatibleRAB[r, a, b],
        If[verbose,
          Print["Compatible triple found --- r=", r, " a=", a, " b=", b]];
        filename = StringForm[prefix<> "`-`-`-`.txt", r,
          Min[a, b], Max[a, b]] // ToString;
        If[verbose, Print["Trying to read from file ", filename]];
        If[FileExistsQ[filename],
          (* the coefficient was computed, get it from the file *)
          If[verbose, Print["File exists, reading solution"]];
          curSol = Get[filename];
        ,
          (* if the coefficient was not computed, do it now*)
          If[verbose, Print["File does not exist, computing solution"]];
          (* preparing the equation to solve for the current coefficient *)
          gg = g;
          For[rr = 0, rr ≤ rmax, rr++,
            For[aa = 0, aa ≤ amax, aa++,
              For[bb = aa, bb ≤ bmax, bb++,
                If[rr > r || (rr == r && aa > a) || (rr == r && aa == a && bb > b),
                  gg = gg /. {c[aa, bb, rr] → 0}];
                ]]];
          If[verbose, Print["Begin... Expand with gg=", gg]];
          ff = f /. {X → W / (1 + W)^2 * (1 + gg)};
          eqs = ff - gg;
          (*If[verbose, Print["Simplifying toExpand..."]];
          toExpand=Simplify[toExpand, W>0&&W<1];*)
          sc = SeriesCoefficient[eqs, {Y, 0, r}, {B, 0, b}, {A, 0, a}];
          If[verbose, Print["...done!"]];
          If[verbose, Print[sc]];
          If[verbose,
            Print["Coefficient r=", r, " a=", a, " b=", b, " computed."]];
          curSol = Solve[0 == sc, c[a, b, r]];
          If[verbose, Print["solutions found: ", curSol]];
          (* we need to find the right solution -
            this is the one starting with W *)
          goodSol = 0;
          For[i = 1, i ≤ Length[curSol], i++,
            If[Limit[(c[a, b, r] /. curSol[[i]]), W → 0] == 0, goodSol = i]];
          If[verbose, Print["Equation solved, correct solution is ", goodSol]];
          curSol = FullSimplify[curSol[[goodSol]], W > 0 && W < 1];
          (* write the coefficient in the file *)
          Put[curSol, filename];
        ];
      ];
    ];
  ];
  Collect[g, {Y, A, B}]
];

```

```

In[1180]:= r = 0;
a = Max[2 * r - 2, 1];
b = Max[2 * r - 2, 1];
ix = Expand[IFromFile[r, a, b]]
Timing[kx = MomentCumulantXYAB[ix, r, a, b, "LX-irred-"]]
Timing[mw = MomentCumulantWYAB[kx, r, a, b, "MW-irred-"]]
SeriesCoefficient[mw /. {A → 1, B → 1}, {Y, 0, r}] // FullSimplify

```

Out[1183]=  $X$

Out[1184]=  $\left\{0.006419, -\frac{X}{-1 + X}\right\}$

Out[1185]=  $\{0.014962, W\}$

Out[1186]=  $W$

```

In[1187]:= r = 1;
a = Max[2 * r - 2, 1];
b = Max[2 * r - 2, 1];
ix = Expand[IFromFile[r, a, b]]
Timing[kx = MomentCumulantXYAB[ix, r, a, b, "LX-irred-"]]
Timing[mw = MomentCumulantWYAB[kx, r, a, b, "MW-irred-"]]
scw = SeriesCoefficient[mw /. {A → 1, B → 1}, {Y, 0, r}] // FullSimplify
ptilde = Expand[scw * (1 - W) ^ (2 * r - 1) / ((1 + W) * W ^ (r + 1)) // FullSimplify]

```

Out[1190]=  $X + A X^2 Y + B X^2 Y$

Out[1191]=  $\left\{0.010591, -\frac{X}{-1 + X} + \left(-\frac{A X^2}{(-1 + X)^3} - \frac{B X^2}{(-1 + X)^3}\right) Y\right\}$

Out[1192]=  $\left\{0.056396, W + \left(-\frac{A W^2 (1 + W)}{-1 + W} - \frac{B W^2 (1 + W)}{-1 + W}\right) Y\right\}$

Out[1193]=  $-\frac{2 W^2 (1 + W)}{-1 + W}$

Out[1194]=  $2$

```

In[1203]:= r = 2;
a = Max[2 * r - 2, 1];
b = Max[2 * r - 2, 1];
ix = Expand[IFromFile[r, a, b]]
Timing[kx = MomentCumulantXYAB[ix, r, a, b, "LX-irred-"]]
Timing[mw = MomentCumulantWYAB[kx, r, a, b, "MW-irred-"]]
scw = SeriesCoefficient[mw /. {A -> 1, B -> 1}, {Y, 0, r}] // FullSimplify
ptilde = Expand[scw * (1 - W) ^ (2 * r - 1) / ((1 + W) * W ^ (r + 1)) // FullSimplify]
    
```

```

Out[1206]= X + A X^2 Y + B X^2 Y + A^2 X^3 Y^2 + 6 A B X^3 Y^2 + B^2 X^3 Y^2 + 2 A B X^4 Y^2 + 2 A^2 B^2 X^4 Y^2
    
```

```

Out[1207]= {0.055261, - X / (-1 + X) + ( - A X^2 / (-1 + X)^3 - B X^2 / (-1 + X)^3 ) Y +
            ( - 6 A B X^3 / (-1 + X)^5 - B^2 X^3 (1 + X) / (-1 + X)^5 + A^2 ( - 2 B^2 X^4 / (-1 + X)^5 - X^3 (1 + X) / (-1 + X)^5 ) ) Y^2 }
    
```

```

Out[1208]= {1.188067, W + ( - A W^2 (1 + W) / (-1 + W) - B W^2 (1 + W) / (-1 + W) ) Y +
            ( B^2 W^3 (-1 - 3 W + 2 W^3) / (-1 + W)^3 - 2 A B W^3 (1 + W) (3 + W (-1 + (-2 + W) W)) / (-1 + W)^3 +
              A^2 ( - 2 B^2 W^4 (1 + W) / (-1 + W) + W^3 (-1 - 3 W + 2 W^3) / (-1 + W)^3 ) ) Y^2 }
    
```

```

Out[1209]= - 4 (-2 + W) W^3 (1 + W) (-1 + (-1 + W) W) / (-1 + W)^3
    
```

```

Out[1210]= 8 + 4 W - 12 W^2 + 4 W^3
    
```

```

In[1211]:= r = 3;
a = Max[2 * r - 2, 1];
b = Max[2 * r - 2, 1];
ix = Expand[IFromFile[r, a, b]]
Timing[kx = MomentCumulantXYAB[ix, r, a, b, "LX-irred-"]]
Timing[mw = MomentCumulantWYAB[kx, r, a, b, "MW-irred-"]]
scw = SeriesCoefficient[mw /. {A -> 1, B -> 1}, {Y, 0, r}] // FullSimplify
ptilde = Expand[scw * (1 - W) ^ (2 * r - 1) / ((1 + W) * W ^ (r + 1)) // FullSimplify]

```

```

Out[1214]= X + A X^2 Y + B X^2 Y + A^2 X^3 Y^2 + 6 A B X^3 Y^2 + B^2 X^3 Y^2 + 2 A B X^4 Y^2 +
2 A^2 B^2 X^4 Y^2 + A^3 X^4 Y^3 + 20 A^2 B X^4 Y^3 + 20 A B^2 X^4 Y^3 + B^3 X^4 Y^3 +
15 A^2 B X^5 Y^3 + 15 A B^2 X^5 Y^3 + 15 A^3 B^2 X^5 Y^3 + 15 A^2 B^3 X^5 Y^3 + 3 A^2 B X^6 Y^3 +
3 A B^2 X^6 Y^3 + 3 A^3 B^2 X^6 Y^3 + 3 A^2 B^3 X^6 Y^3 + 3 A^4 B^3 X^6 Y^3 + 3 A^3 B^4 X^6 Y^3

```

$$\begin{aligned}
\text{Out[1215]} = & \left\{ 0.078444, -\frac{X}{-1+X} + \left( -\frac{A X^2}{(-1+X)^3} - \frac{B X^2}{(-1+X)^3} \right) Y + \right. \\
& \left( -\frac{6 A B X^3}{(-1+X)^5} - \frac{B^2 X^3 (1+X)}{(-1+X)^5} + A^2 \left( -\frac{2 B^2 X^4}{(-1+X)^5} - \frac{X^3 (1+X)}{(-1+X)^5} \right) \right) Y^2 + \\
& \left( -\frac{3 A^4 B^3 X^6}{(-1+X)^7} - \frac{10 A B^2 X^4 (2+X)}{(-1+X)^7} + A^2 \left( -\frac{15 B^3 X^5}{(-1+X)^7} - \frac{10 B X^4 (2+X)}{(-1+X)^7} \right) - \right. \\
& \left. \frac{B^3 X^4 (1+X (3+X))}{(-1+X)^7} + A^3 \left( -\frac{15 B^2 X^5}{(-1+X)^7} - \frac{3 B^4 X^6}{(-1+X)^7} - \frac{X^4 (1+X (3+X))}{(-1+X)^7} \right) \right) Y^3 \Big\}
\end{aligned}$$

$$\begin{aligned}
\text{Out[1216]} = & \left\{ 9.029903, W + \left( -\frac{A W^2 (1+W)}{-1+W} - \frac{B W^2 (1+W)}{-1+W} \right) Y + \right. \\
& \left( \frac{B^2 W^3 (-1-3W+2W^3)}{(-1+W)^3} - \frac{2 A B W^3 (1+W) (3+W (-1+(-2+W) W))}{(-1+W)^3} + \right. \\
& \left. A^2 \left( -\frac{2 B^2 W^4 (1+W)}{-1+W} + \frac{W^3 (-1-3W+2W^3)}{(-1+W)^3} \right) \right) Y^2 + \\
& \left( -\frac{3 A^4 B^3 W^6 (1+W)}{-1+W} - \frac{B^3 W^4 (1+W) (1+W (6+5 (-2+W) W^2))}{(-1+W)^5} + A^3 \left( -\frac{3 B^4 W^6 (1+W)}{-1+W} - \right. \right. \\
& \left. \frac{W^4 (1+W) (1+W (6+5 (-2+W) W^2))}{(-1+W)^5} - \frac{B^2 W^5 (1+W) (15+W (-3+W (-11+3W)))}{(-1+W)^3} \right) - \\
& \frac{1}{(-1+W)^5} A B^2 W^4 (1+W) (20+W (5+W (-43+W (16+(-2+W) W (-11+3W)))))) + \\
& A^2 \left( -\frac{B^3 W^5 (1+W) (15+W (-3+W (-11+3W)))}{(-1+W)^3} - \frac{1}{(-1+W)^5} \right. \\
& \left. \left. B W^4 (1+W) (20+W (5+W (-43+W (16+(-2+W) W (-11+3W)))) \right) \right) \right) Y^3 \Big\}
\end{aligned}$$

$$\text{Out[1217]} = -\frac{1}{(-1+W)^5} 2 W^4 (1+W) (-1+(-2+W) W) (-21+W (16+(-2+W) W (-10+9W)))$$

$$\text{Out[1218]} = 42 + 52 W - 146 W^2 + 8 W^3 + 134 W^4 - 92 W^5 + 18 W^6$$

```

In[1219]:= r = 4;
a = Max[2 * r - 2, 1];
b = Max[2 * r - 2, 1];
ix = Expand[IFromFile[r, a, b]]
Timing[kx = MomentCumulantXYAB[ix, r, a, b, "LX-irred-"]]
Timing[mw = MomentCumulantWYAB[kx, r, a, b, "MW-irred-"]]
scw = SeriesCoefficient[mw /. {A -> 1, B -> 1}, {Y, 0, r}] // FullSimplify
ptilde = Expand[scw * (1 - W) ^ (2 * r - 1) / ((1 + W) * W ^ (r + 1)) // FullSimplify]
    
```

```

Out[1222]= X + A X^2 Y + B X^2 Y + A^2 X^3 Y^2 + 6 A B X^3 Y^2 + B^2 X^3 Y^2 + 2 A B X^4 Y^2 + 2 A^2 B^2 X^4 Y^2 + A^3 X^4 Y^3 +
20 A^2 B X^4 Y^3 + 20 A B^2 X^4 Y^3 + B^3 X^4 Y^3 + 15 A^2 B X^5 Y^3 + 15 A B^2 X^5 Y^3 + 15 A^3 B^2 X^5 Y^3 +
15 A^2 B^3 X^5 Y^3 + 3 A^2 B X^6 Y^3 + 3 A B^2 X^6 Y^3 + 3 A^3 B^2 X^6 Y^3 + 3 A^2 B^3 X^6 Y^3 + 3 A^4 B^3 X^6 Y^3 +
3 A^3 B^4 X^6 Y^3 + A^4 X^5 Y^4 + 50 A^3 B X^5 Y^4 + 160 A^2 B^2 X^5 Y^4 + 50 A B^3 X^5 Y^4 + B^4 X^5 Y^4 +
63 A^3 B X^6 Y^4 + 224 A^2 B^2 X^6 Y^4 + 63 A^4 B^2 X^6 Y^4 + 63 A B^3 X^6 Y^4 + 224 A^3 B^3 X^6 Y^4 +
63 A^2 B^4 X^6 Y^4 + 28 A^3 B X^7 Y^4 + 112 A^2 B^2 X^7 Y^4 + 28 A^4 B^2 X^7 Y^4 + 28 A B^3 X^7 Y^4 +
126 A^3 B^3 X^7 Y^4 + 28 A^5 B^3 X^7 Y^4 + 28 A^2 B^4 X^7 Y^4 + 112 A^4 B^4 X^7 Y^4 + 28 A^3 B^5 X^7 Y^4 +
4 A^3 B X^8 Y^4 + 20 A^2 B^2 X^8 Y^4 + 4 A^4 B^2 X^8 Y^4 + 4 A B^3 X^8 Y^4 + 20 A^3 B^3 X^8 Y^4 + 4 A^5 B^3 X^8 Y^4 +
4 A^2 B^4 X^8 Y^4 + 20 A^4 B^4 X^8 Y^4 + 4 A^6 B^4 X^8 Y^4 + 4 A^3 B^5 X^8 Y^4 + 20 A^5 B^5 X^8 Y^4 + 4 A^4 B^6 X^8 Y^4
    
```

```

Out[1223]= {6.513344, - X / (-1 + X) + (- A X^2 / (-1 + X)^3 - B X^2 / (-1 + X)^3) Y +
(- 6 A B X^3 / (-1 + X)^5 - B^2 X^3 (1 + X) / (-1 + X)^5 + A^2 (- 2 B^2 X^4 / (-1 + X)^5 - X^3 (1 + X) / (-1 + X)^5)) Y^2 +
(- 3 A^4 B^3 X^6 / (-1 + X)^7 - 10 A B^2 X^4 (2 + X) / (-1 + X)^7 + A^2 (- 15 B^3 X^5 / (-1 + X)^7 - 10 B X^4 (2 + X) / (-1 + X)^7) -
B^3 X^4 (1 + X (3 + X)) / (-1 + X)^7 + A^3 (- 15 B^2 X^5 / (-1 + X)^7 - 3 B^4 X^6 / (-1 + X)^7 - X^4 (1 + X (3 + X)) / (-1 + X)^7) Y^3 +
(- 4 A^6 B^4 X^8 / (-1 + X)^9 + A^5 (- 28 B^3 X^7 / (-1 + X)^9 - 20 B^5 X^8 / (-1 + X)^9) - B^4 X^5 (1 + X) (1 + X (5 + X)) / (-1 + X)^9 -
5 A B^3 X^5 (10 + 3 X (5 + X)) / (-1 + X)^9 +
A^4 (28 B^4 (-4 + X) X^7 / (-1 + X)^9 - 4 B^6 X^8 / (-1 + X)^9 - 21 B^2 X^6 (3 + X) / (-1 + X)^9 - X^5 (1 + X) (1 + X (5 + X)) / (-1 + X)^9) +
A^3 (- 28 B^5 X^7 / (-1 + X)^9 - 5 B X^5 (10 + 3 X (5 + X)) / (-1 + X)^9 - 4 B^3 X^6 (56 + X (-7 + 4 X)) / (-1 + X)^9) +
A^2 (- 21 B^4 X^6 (3 + X) / (-1 + X)^9 + 2 B^2 X^5 (-80 + X (-49 + (-12 + X) X)) / (-1 + X)^9) Y^4}
    
```

```

Out[1224]= {52.620197, W + (- A W^2 (1 + W) / (-1 + W) - B W^2 (1 + W) / (-1 + W)) Y +
(B^2 W^3 (-1 - 3 W + 2 W^3) / (-1 + W)^3 - 2 A B W^3 (1 + W) (3 + W (-1 + (-2 + W) W)) / (-1 + W)^3 +
A^2 (- 2 B^2 W^4 (1 + W) / (-1 + W) + W^3 (-1 - 3 W + 2 W^3) / (-1 + W)^3)) Y^2 +
    
```

$$\begin{aligned}
& \left( -\frac{3 A^4 B^3 W^6 (1+W)}{-1+W} - \frac{B^3 W^4 (1+W) (1+W (6+5 (-2+W) W^2))}{(-1+W)^5} + A^3 \left( -\frac{3 B^4 W^6 (1+W)}{-1+W} - \right. \right. \\
& \quad \left. \frac{W^4 (1+W) (1+W (6+5 (-2+W) W^2))}{(-1+W)^5} - \frac{B^2 W^5 (1+W) (15+W (-3+W (-11+3 W)))}{(-1+W)^3} \right) - \\
& \quad \frac{1}{(-1+W)^5} A B^2 W^4 (1+W) (20+W (5+W (-43+W (16+(-2+W) W (-11+3 W)))) + \\
& \quad A^2 \left( -\frac{B^3 W^5 (1+W) (15+W (-3+W (-11+3 W)))}{(-1+W)^3} - \frac{1}{(-1+W)^5} \right. \\
& \quad \left. \left. B W^4 (1+W) (20+W (5+W (-43+W (16+(-2+W) W (-11+3 W)))) \right) \right) \right) Y^3 + \\
& \left( -\frac{4 A^6 B^4 W^8 (1+W)}{-1+W} + A^5 \left( -\frac{20 B^5 W^8 (1+W)}{-1+W} - \frac{2 B^3 W^7 (1+W) (14+W (-2+W (-11+2 W)))}{(-1+W)^3} \right) + \right. \\
& \quad \frac{1}{(-1+W)^7} B^4 W^5 (1+W) (-1+W (-12+W (-19+W (34+7 W (3+2 (-3+W) W)))) + \\
& \quad A^4 \left( -\frac{4 B^6 W^8 (1+W)}{-1+W} - \frac{4 B^4 W^7 (1+W) (28+W (-19+5 (-2+W) W))}{(-1+W)^3} + \frac{1}{(-1+W)^7} \right. \\
& \quad \left. W^5 (1+W) (-1+W (-12+W (-19+W (34+7 W (3+2 (-3+W) W)))) - \frac{1}{(-1+W)^5} \right. \\
& \quad \left. B^2 W^6 (1+W) (63+W (14+W (-122+W (24+W (59-30 W+4 W^2)))) \right) \right) + \\
& \quad A^2 \left( -\frac{1}{(-1+W)^5} B^4 W^6 (1+W) (63+W (14+W (-122+W (24+W (59-30 W+4 W^2)))) - \right. \\
& \quad \frac{1}{(-1+W)^7} 2 B^2 W^5 (1+W) (80+W (-14+ \\
& \quad \left. W (-196+W (100+(-2+W) W (-116+W (63+2 W (19+5 (-4+W) W)))) \right) \right) - \\
& \quad \frac{1}{(-1+W)^7} A B^3 W^5 (1+W) (50+W (87+W (-200+W (-79+W (324+ \\
& \quad \left. W (-127+W (-124+W (123-38 W+4 W^2)))) \right) \right) + \\
& \quad A^3 \left( -\frac{2 B^5 W^7 (1+W) (14+W (-2+W (-11+2 W)))}{(-1+W)^3} - \frac{1}{(-1+W)^5} 2 B^3 W^6 (1+W) \right. \\
& \quad \left. (112+W (-91+W (-90+W (74+W (44+W (-47+10 W)))) \right) - \\
& \quad \frac{1}{(-1+W)^7} B W^5 (1+W) (50+W (87+W (-200+ \\
& \quad \left. W (-79+W (324+W (-127+W (-124+W (123-38 W+4 W^2)))) \right) \right) \right) \right) Y^4 \} \\
& \text{Out[1225]= } -\frac{1}{(-1+W)^7} 2 W^5 (1+W) (131+W (260+ \\
& \quad W (-720+W (-260+W (1526+W (-828+W (-672+W (932+7 W (-55+8 W)))) \right) \right) \\
& \text{Out[1226]= } 262+520 W-1440 W^2-520 W^3+3052 W^4-1656 W^5-1344 W^6+1864 W^7-770 W^8+112 W^9
\end{aligned}$$



```

In[1227]:= r = 5;
a = Max[2 * r - 2, 1];
b = Max[2 * r - 2, 1];
ix = Expand[IFromFile[r, a, b]]
Timing[kx = MomentCumulantXYAB[ix, r, a, b, "LX-irred-"]]
Timing[mw = MomentCumulantWYAB[kx, r, a, b, "MW-irred-"]]
scw = SeriesCoefficient[mw /. {A -> 1, B -> 1}, {Y, 0, r}] // FullSimplify
ptilde = Expand[scw * (1 - W) ^ (2 * r - 1) / ((1 + W) * W ^ (r + 1))] // FullSimplify

Out[1230]= X + A X^2 Y + B X^2 Y + A^2 X^3 Y^2 + 6 A B X^3 Y^2 + B^2 X^3 Y^2 + 2 A B X^4 Y^2 + 2 A^2 B^2 X^4 Y^2 + A^3 X^4 Y^3 +
20 A^2 B X^4 Y^3 + 20 A B^2 X^4 Y^3 + B^3 X^4 Y^3 + 15 A^2 B X^5 Y^3 + 15 A B^2 X^5 Y^3 + 15 A^3 B^2 X^5 Y^3 +
15 A^2 B^3 X^5 Y^3 + 3 A^2 B X^6 Y^3 + 3 A B^2 X^6 Y^3 + 3 A^3 B^2 X^6 Y^3 + 3 A^2 B^3 X^6 Y^3 + 3 A^4 B^3 X^6 Y^3 +
3 A^3 B^4 X^6 Y^3 + A^4 X^5 Y^4 + 50 A^3 B X^5 Y^4 + 160 A^2 B^2 X^5 Y^4 + 50 A B^3 X^5 Y^4 + B^4 X^5 Y^4 +
63 A^3 B X^6 Y^4 + 224 A^2 B^2 X^6 Y^4 + 63 A^4 B^2 X^6 Y^4 + 63 A B^3 X^6 Y^4 + 224 A^3 B^3 X^6 Y^4 + 63 A^2 B^4 X^6 Y^4 +
28 A^3 B X^7 Y^4 + 112 A^2 B^2 X^7 Y^4 + 28 A^4 B^2 X^7 Y^4 + 28 A B^3 X^7 Y^4 + 126 A^3 B^3 X^7 Y^4 + 28 A^5 B^3 X^7 Y^4 +
28 A^2 B^4 X^7 Y^4 + 112 A^4 B^4 X^7 Y^4 + 28 A^3 B^5 X^7 Y^4 + 4 A^3 B X^8 Y^4 + 20 A^2 B^2 X^8 Y^4 + 4 A^4 B^2 X^8 Y^4 +
4 A B^3 X^8 Y^4 + 20 A^3 B^3 X^8 Y^4 + 4 A^5 B^3 X^8 Y^4 + 4 A^2 B^4 X^8 Y^4 + 20 A^4 B^4 X^8 Y^4 + 4 A^6 B^4 X^8 Y^4 +
4 A^3 B^5 X^8 Y^4 + 20 A^5 B^5 X^8 Y^4 + 4 A^4 B^6 X^8 Y^4 + A^5 X^6 Y^5 + 105 A^4 B X^6 Y^5 + 808 A^3 B^2 X^6 Y^5 +
808 A^2 B^3 X^6 Y^5 + 105 A B^4 X^6 Y^5 + B^5 X^6 Y^5 + 196 A^4 B X^7 Y^5 + 1687 A^3 B^2 X^7 Y^5 + 196 A^5 B^2 X^7 Y^5 +
1687 A^2 B^3 X^7 Y^5 + 1687 A^4 B^3 X^7 Y^5 + 196 A B^4 X^7 Y^5 + 1687 A^3 B^4 X^7 Y^5 + 196 A^2 B^5 X^7 Y^5 +
144 A^4 B X^8 Y^5 + 1392 A^3 B^2 X^8 Y^5 + 144 A^5 B^2 X^8 Y^5 + 1392 A^2 B^3 X^8 Y^5 + 1624 A^4 B^3 X^8 Y^5 +
144 A^6 B^3 X^8 Y^5 + 144 A B^4 X^8 Y^5 + 1624 A^3 B^4 X^8 Y^5 + 1392 A^5 B^4 X^8 Y^5 + 144 A^2 B^5 X^8 Y^5 +
1392 A^4 B^5 X^8 Y^5 + 144 A^3 B^6 X^8 Y^5 + 45 A^4 B X^9 Y^5 + 525 A^3 B^2 X^9 Y^5 + 45 A^5 B^2 X^9 Y^5 +
525 A^2 B^3 X^9 Y^5 + 594 A^4 B^3 X^9 Y^5 + 45 A^6 B^3 X^9 Y^5 + 45 A B^4 X^9 Y^5 + 594 A^3 B^4 X^9 Y^5 +
594 A^5 B^4 X^9 Y^5 + 45 A^7 B^4 X^9 Y^5 + 45 A^2 B^5 X^9 Y^5 + 594 A^4 B^5 X^9 Y^5 + 525 A^6 B^5 X^9 Y^5 +
45 A^3 B^6 X^9 Y^5 + 525 A^5 B^6 X^9 Y^5 + 45 A^4 B^7 X^9 Y^5 + 5 A^4 B X^10 Y^5 + 75 A^3 B^2 X^10 Y^5 + 5 A^5 B^2 X^10 Y^5 +
75 A^2 B^3 X^10 Y^5 + 80 A^4 B^3 X^10 Y^5 + 5 A^6 B^3 X^10 Y^5 + 5 A B^4 X^10 Y^5 + 80 A^3 B^4 X^10 Y^5 +
75 A^5 B^4 X^10 Y^5 + 5 A^7 B^4 X^10 Y^5 + 5 A^2 B^5 X^10 Y^5 + 75 A^4 B^5 X^10 Y^5 + 80 A^6 B^5 X^10 Y^5 + 5 A^8 B^5 X^10 Y^5 +
5 A^3 B^6 X^10 Y^5 + 80 A^5 B^6 X^10 Y^5 + 75 A^7 B^6 X^10 Y^5 + 5 A^4 B^7 X^10 Y^5 + 75 A^6 B^7 X^10 Y^5 + 5 A^5 B^8 X^10 Y^5

```

$$\begin{aligned}
\text{Out[1231]} = & \left\{ 14.822615, -\frac{X}{-1+X} + \left( -\frac{A X^2}{(-1+X)^3} - \frac{B X^2}{(-1+X)^3} \right) Y + \right. \\
& \left( -\frac{6 A B X^3}{(-1+X)^5} - \frac{B^2 X^3 (1+X)}{(-1+X)^5} + A^2 \left( -\frac{2 B^2 X^4}{(-1+X)^5} - \frac{X^3 (1+X)}{(-1+X)^5} \right) \right) Y^2 + \\
& \left( -\frac{3 A^4 B^3 X^6}{(-1+X)^7} - \frac{10 A B^2 X^4 (2+X)}{(-1+X)^7} + A^2 \left( -\frac{15 B^3 X^5}{(-1+X)^7} - \frac{10 B X^4 (2+X)}{(-1+X)^7} \right) - \right. \\
& \left. \frac{B^3 X^4 (1+X (3+X))}{(-1+X)^7} + A^3 \left( -\frac{15 B^2 X^5}{(-1+X)^7} - \frac{3 B^4 X^6}{(-1+X)^7} - \frac{X^4 (1+X (3+X))}{(-1+X)^7} \right) \right) Y^3 + \\
& \left( -\frac{4 A^6 B^4 X^8}{(-1+X)^9} + A^5 \left( -\frac{28 B^3 X^7}{(-1+X)^9} - \frac{20 B^5 X^8}{(-1+X)^9} \right) - \frac{B^4 X^5 (1+X (1+X (5+X)))}{(-1+X)^9} - \right. \\
& \left. \frac{5 A B^3 X^5 (10+3 X (5+X))}{(-1+X)^9} + \right. \\
& A^4 \left( \frac{28 B^4 (-4+X) X^7}{(-1+X)^9} - \frac{4 B^6 X^8}{(-1+X)^9} - \frac{21 B^2 X^6 (3+X)}{(-1+X)^9} - \frac{X^5 (1+X (1+X (5+X)))}{(-1+X)^9} \right) + \\
& A^3 \left( -\frac{28 B^5 X^7}{(-1+X)^9} - \frac{5 B X^5 (10+3 X (5+X))}{(-1+X)^9} - \frac{4 B^3 X^6 (56+X (-7+4 X))}{(-1+X)^9} \right) + \\
& A^2 \left( -\frac{21 B^4 X^6 (3+X)}{(-1+X)^9} + \frac{2 B^2 X^5 (-80+X (-49+(-12+X) X))}{(-1+X)^9} \right) \Big) Y^4 + \\
& \left( -\frac{5 A^8 B^5 X^{10}}{(-1+X)^{11}} + A^7 \left( -\frac{45 B^4 X^9}{(-1+X)^{11}} - \frac{75 B^6 X^{10}}{(-1+X)^{11}} \right) + \right. \\
& A^6 \left( -\frac{75 B^7 X^{10}}{(-1+X)^{11}} - \frac{36 B^3 X^8 (4+X)}{(-1+X)^{11}} + \frac{5 B^5 X^9 (-105+29 X)}{(-1+X)^{11}} \right) - \\
& \frac{21 A B^4 X^6 (5+X (15+X (9+X)))}{(-1+X)^{11}} - \frac{B^5 X^6 (1+X (10+X (20+X (10+X))))}{(-1+X)^{11}} + \\
& A^2 \left( -\frac{28 B^5 X^7 (7+X (7+X))}{(-1+X)^{11}} - \frac{4 B^3 X^6 (202+X (228+X (93+2 X)))}{(-1+X)^{11}} \right) + \\
& A^4 \left( -\frac{45 B^7 X^9}{(-1+X)^{11}} - \frac{3 B^5 X^8 (464+X (-157+33 X))}{(-1+X)^{11}} - \frac{21 B X^6 (5+X (15+X (9+X)))}{(-1+X)^{11}} + \right. \\
& \left. \frac{B^3 X^7 (-1687+X (-19+X (-238+19 X)))}{(-1+X)^{11}} \right) + A^3 \left( -\frac{36 B^6 X^8 (4+X)}{(-1+X)^{11}} - \right. \\
& \left. \frac{4 B^2 X^6 (202+X (228+X (93+2 X)))}{(-1+X)^{11}} + \frac{B^4 X^7 (-1687+X (-19+X (-238+19 X)))}{(-1+X)^{11}} \right) + \\
& A^5 \left( -\frac{5 B^8 X^{10}}{(-1+X)^{11}} + \frac{5 B^6 X^9 (-105+29 X)}{(-1+X)^{11}} - \frac{28 B^2 X^7 (7+X (7+X))}{(-1+X)^{11}} - \right. \\
& \left. \frac{3 B^4 X^8 (464+X (-157+33 X))}{(-1+X)^{11}} - \frac{X^6 (1+X (10+X (20+X (10+X))))}{(-1+X)^{11}} \right) \Big) Y^5 \Big\} \\
\text{Out[1232]} = & \left\{ 197.145030, W + \left( -\frac{A W^2 (1+W)}{-1+W} - \frac{B W^2 (1+W)}{-1+W} \right) Y + \right.
\end{aligned}$$

$$\begin{aligned}
 & \left( \frac{B^2 W^3 (-1 - 3W + 2W^3)}{(-1 + W)^3} - \frac{2ABW^3(1 + W)(3 + W(-1 + (-2 + W)W))}{(-1 + W)^3} + \right. \\
 & \quad \left. A^2 \left( -\frac{2B^2 W^4(1 + W)}{-1 + W} + \frac{W^3(-1 - 3W + 2W^3)}{(-1 + W)^3} \right) \right) Y^2 + \\
 & \left( -\frac{3A^4 B^3 W^6(1 + W)}{-1 + W} - \frac{B^3 W^4(1 + W)(1 + W(6 + 5(-2 + W)W^2))}{(-1 + W)^5} + A^3 \left( -\frac{3B^4 W^6(1 + W)}{-1 + W} - \right. \right. \\
 & \quad \left. \frac{W^4(1 + W)(1 + W(6 + 5(-2 + W)W^2))}{(-1 + W)^5} - \frac{B^2 W^5(1 + W)(15 + W(-3 + W(-11 + 3W)))}{(-1 + W)^3} \right) - \\
 & \quad \frac{1}{(-1 + W)^5} AB^2 W^4(1 + W)(20 + W(5 + W(-43 + W(16 + (-2 + W)W(-11 + 3W)))) + \\
 & \quad \left. A^2 \left( -\frac{B^3 W^5(1 + W)(15 + W(-3 + W(-11 + 3W)))}{(-1 + W)^3} - \frac{1}{(-1 + W)^5} \right. \right. \\
 & \quad \left. \left. BW^4(1 + W)(20 + W(5 + W(-43 + W(16 + (-2 + W)W(-11 + 3W)))) \right) \right) Y^3 + \\
 & \left( -\frac{4A^6 B^4 W^8(1 + W)}{-1 + W} + A^5 \left( -\frac{20B^5 W^8(1 + W)}{-1 + W} - \frac{2B^3 W^7(1 + W)(14 + W(-2 + W(-11 + 2W)))}{(-1 + W)^3} \right) \right) + \\
 & \quad \frac{1}{(-1 + W)^7} B^4 W^5(1 + W)(-1 + W(-12 + W(-19 + W(34 + 7W(3 + 2(-3 + W)W)))) + \\
 & \quad A^4 \left( -\frac{4B^6 W^8(1 + W)}{-1 + W} - \frac{4B^4 W^7(1 + W)(28 + W(-19 + 5(-2 + W)W))}{(-1 + W)^3} + \frac{1}{(-1 + W)^7} \right. \\
 & \quad \left. W^5(1 + W)(-1 + W(-12 + W(-19 + W(34 + 7W(3 + 2(-3 + W)W)))) - \frac{1}{(-1 + W)^5} \right. \\
 & \quad \left. B^2 W^6(1 + W)(63 + W(14 + W(-122 + W(24 + W(59 - 30W + 4W^2)))) \right) + \\
 & \quad A^2 \left( -\frac{1}{(-1 + W)^5} B^4 W^6(1 + W)(63 + W(14 + W(-122 + W(24 + W(59 - 30W + 4W^2)))) - \right. \\
 & \quad \frac{1}{(-1 + W)^7} 2B^2 W^5(1 + W)(80 + W(-14 + \\
 & \quad \left. W(-196 + W(100 + (-2 + W)W(-116 + W(63 + 2W(19 + 5(-4 + W)W)))) \right) - \\
 & \quad \frac{1}{(-1 + W)^7} AB^3 W^5(1 + W)(50 + W(87 + W(-200 + W(-79 + W(324 + \\
 & \quad \left. W(-127 + W(-124 + W(123 - 38W + 4W^2)))) \right) + \\
 & \quad A^3 \left( -\frac{2B^5 W^7(1 + W)(14 + W(-2 + W(-11 + 2W)))}{(-1 + W)^3} - \frac{1}{(-1 + W)^5} 2B^3 W^6(1 + W) \right. \\
 & \quad \left. (112 + W(-91 + W(-90 + W(74 + W(44 + W(-47 + 10W)))) \right) - \\
 & \quad \frac{1}{(-1 + W)^7} B W^5(1 + W)(50 + W(87 + W(-200 + \\
 & \quad \left. W(-79 + W(324 + W(-127 + W(-124 + W(123 - 38W + 4W^2)))) \right) \right) Y^4 +
 \end{aligned}$$

$$\begin{aligned}
& \left( -\frac{5 A^8 B^5 W^{10} (1+W)}{-1+W} + A^7 \left( -\frac{75 B^6 W^{10} (1+W)}{-1+W} - \frac{B^4 W^9 (1+W) (45+W (-5+W (-37+5 W)))}{(-1+W)^3} \right) + \right. \\
& A^6 \left( -\frac{75 B^7 W^{10} (1+W)}{-1+W} - \frac{5 B^5 (-3+W) W^9 (1+W) (-35+W (13+16 W))}{(-1+W)^3} - \frac{1}{(-1+W)^5} B^3 W^8 \right. \\
& \quad \left. (1+W) (144+W (27+W (-273+W (32+W (130+W (-47+5 W)))))) \right) - \frac{1}{(-1+W)^9} \\
& B^5 W^6 (1+W (21+W (96+W (56+W (-237+7 W (-15+2 W (20+3 (-3+W) W^2)))))) + \\
& A^5 \left( -\frac{5 B^8 W^{10} (1+W)}{-1+W} - \frac{5 B^6 (-3+W) W^9 (1+W) (-35+W (13+16 W))}{(-1+W)^3} - \frac{1}{(-1+W)^5} B^4 W^8 (1+W) \right. \\
& \quad \left. (1392+W (-1536+W (-691+W (998+W (194-354 W+75 W^2)))) \right) - \frac{1}{(-1+W)^9} \\
& W^6 (1+W (21+W (96+W (56+W (-237+7 W (-15+2 W (20+3 (-3+W) W^2)))))) - \\
& \frac{1}{(-1+W)^7} B^2 W^7 (1+W) (196+W (248+W (-654+W (-265+W (863+ \\
& \quad W (-201+(-4+W) W (81+W (-37+5 W)))))) \right) - \frac{1}{(-1+W)^9} A B^4 \\
& W^6 (1+W) (105+W (434+W (-396+W (-1296+W (1664+W (817+W (-2372+W (991+ \\
& \quad W (676+W (-839+W (348+W (-67+5 W))))))))) + \\
& A^4 \left( -\frac{B^7 W^9 (1+W) (45+W (-5+W (-37+5 W)))}{(-1+W)^3} - \frac{1}{(-1+W)^5} B^5 W^8 (1+W) \right. \\
& \quad \left. (1392+W (-1536+W (-691+W (998+W (194-354 W+75 W^2)))) \right) - \\
& \frac{1}{(-1+W)^7} B^3 W^7 (1+W) (1687+W (-1586+W (-2142+W (2176+ \\
& \quad W (1977+2 W (-1305+W (-26+W (562+W (-267+40 W)))))) \right) - \\
& \frac{1}{(-1+W)^9} B W^6 (1+W) (105+W (434+W (-396+W (-1296+W (1664+ \\
& \quad W (817+W (-2372+W (991+W (676+W (-839+ \\
& \quad W (348+W (-67+5 W))))))))) \right) + A^3 \\
& \left( -\frac{1}{(-1+W)^5} B^6 W^8 (1+W) (144+W (27+W (-273+W (32+W (130+W (-47+5 W)))))) - \right. \\
& \frac{1}{(-1+W)^7} B^4 W^7 (1+W) (1687+W (-1586+W (-2142+W (2176+ \\
& \quad W (1977+2 W (-1305+W (-26+W (562+W (-267+40 W)))))) \right) - \\
& \frac{1}{(-1+W)^9} B^2 W^6 (1+W) (808+W (137+W (-2944+W (806+W (5821+ \\
& \quad W (-5191+W (-3236+W (6665+W (-2180+W (-1850+ \\
& \quad W (1844+15 W (-41+5 W))))))))) \right) + \\
& A^2 \left( -\frac{1}{(-1+W)^7} B^5 W^7 (1+W) (196+W (248+W (-654+W (-265+W (863+ \\
& \quad W (-201+(-4+W) W (81+W (-37+5 W)))))) \right) -
\end{aligned}$$

$$\frac{1}{(-1+W)^9} B^3 W^6 (1+W) (808+W (137+W (-2944+W (806+W (5821+W (-5191+W (-3236+W (6665+W (-2180+W (-1850+W (1844+15 W (-41+5 W)))))))))) \Bigg) \Bigg) Y^5 \Bigg\}$$

$$\text{Out[1233]} = -\frac{1}{(-1+W)^9} 4 W^6 (1+W) (457+W (1237+W (-3416+W (-2915+W (12003+W (-4202+W (-13728+W (15142+W (-777+W (-7947+W (5816+41 W (-43+5 W))))))))))$$

$$\text{Out[1234]} = 1828 + 4948 W - 13664 W^2 - 11660 W^3 + 48012 W^4 - 16808 W^5 - 54912 W^6 + 60568 W^7 - 3108 W^8 - 31788 W^9 + 23264 W^{10} - 7052 W^{11} + 820 W^{12}$$

```

In[1263]:= r = 6;
a = Max[2 * r - 2, 1];
b = Max[2 * r - 2, 1];
ix = Expand[IFromFile[r, a, b]]
Timing[kx = MomentCumulantXYAB[ix, r, a, b, "LX-irred-"]]
Timing[mw = MomentCumulantWYAB[kx, r, a, b, "MW-irred-"]]
scw = SeriesCoefficient[mw /. {A -> 1, B -> 1}, {Y, 0, r}] // FullSimplify
ptilde =
FullSimplify[scw * (1 - W) ^ (2 * r - 1) / ((1 + W) * W ^ (r + 1)), W > 0 && W < 1] // Factor //
Expand

```

$$\begin{aligned}
\text{Out[1266]} = & X + A X^2 Y + B X^2 Y + A^2 X^3 Y^2 + 6 A B X^3 Y^2 + B^2 X^3 Y^2 + 2 A B X^4 Y^2 + 2 A^2 B^2 X^4 Y^2 + A^3 X^4 Y^3 + \\
& 20 A^2 B X^4 Y^3 + 20 A B^2 X^4 Y^3 + B^3 X^4 Y^3 + 15 A^2 B X^5 Y^3 + 15 A B^2 X^5 Y^3 + 15 A^3 B^2 X^5 Y^3 + \\
& 15 A^2 B^3 X^5 Y^3 + 3 A^2 B X^6 Y^3 + 3 A B^2 X^6 Y^3 + 3 A^3 B^2 X^6 Y^3 + 3 A^2 B^3 X^6 Y^3 + 3 A^4 B^3 X^6 Y^3 + \\
& 3 A^3 B^4 X^6 Y^3 + A^4 X^5 Y^4 + 50 A^3 B X^5 Y^4 + 160 A^2 B^2 X^5 Y^4 + 50 A B^3 X^5 Y^4 + B^4 X^5 Y^4 + \\
& 63 A^3 B X^6 Y^4 + 224 A^2 B^2 X^6 Y^4 + 63 A^4 B^2 X^6 Y^4 + 63 A B^3 X^6 Y^4 + 224 A^3 B^3 X^6 Y^4 + \\
& 63 A^2 B^4 X^6 Y^4 + 28 A^3 B X^7 Y^4 + 112 A^2 B^2 X^7 Y^4 + 28 A^4 B^2 X^7 Y^4 + 28 A B^3 X^7 Y^4 + \\
& 126 A^3 B^3 X^7 Y^4 + 28 A^5 B^3 X^7 Y^4 + 28 A^2 B^4 X^7 Y^4 + 112 A^4 B^4 X^7 Y^4 + 28 A^3 B^5 X^7 Y^4 + \\
& 4 A^3 B X^8 Y^4 + 20 A^2 B^2 X^8 Y^4 + 4 A^4 B^2 X^8 Y^4 + 4 A B^3 X^8 Y^4 + 20 A^3 B^3 X^8 Y^4 + 4 A^5 B^3 X^8 Y^4 + \\
& 4 A^2 B^4 X^8 Y^4 + 20 A^4 B^4 X^8 Y^4 + 4 A^6 B^4 X^8 Y^4 + 4 A^3 B^5 X^8 Y^4 + 20 A^5 B^5 X^8 Y^4 + 4 A^4 B^6 X^8 Y^4 + \\
& A^5 X^6 Y^5 + 105 A^4 B X^6 Y^5 + 808 A^3 B^2 X^6 Y^5 + 808 A^2 B^3 X^6 Y^5 + 105 A B^4 X^6 Y^5 + B^5 X^6 Y^5 + \\
& 196 A^4 B X^7 Y^5 + 1687 A^3 B^2 X^7 Y^5 + 196 A^5 B^2 X^7 Y^5 + 1687 A^2 B^3 X^7 Y^5 + 1687 A^4 B^3 X^7 Y^5 + \\
& 196 A B^4 X^7 Y^5 + 1687 A^3 B^4 X^7 Y^5 + 196 A^2 B^5 X^7 Y^5 + 144 A^4 B X^8 Y^5 + 1392 A^3 B^2 X^8 Y^5 + \\
& 144 A^5 B^2 X^8 Y^5 + 1392 A^2 B^3 X^8 Y^5 + 1624 A^4 B^3 X^8 Y^5 + 144 A^6 B^3 X^8 Y^5 + 144 A B^4 X^8 Y^5 + \\
& 1624 A^3 B^4 X^8 Y^5 + 1392 A^5 B^4 X^8 Y^5 + 144 A^2 B^5 X^8 Y^5 + 1392 A^4 B^5 X^8 Y^5 + 144 A^3 B^6 X^8 Y^5 + \\
& 45 A^4 B X^9 Y^5 + 525 A^3 B^2 X^9 Y^5 + 45 A^5 B^2 X^9 Y^5 + 525 A^2 B^3 X^9 Y^5 + 594 A^4 B^3 X^9 Y^5 + \\
& 45 A^6 B^3 X^9 Y^5 + 45 A B^4 X^9 Y^5 + 594 A^3 B^4 X^9 Y^5 + 594 A^5 B^4 X^9 Y^5 + 45 A^7 B^4 X^9 Y^5 + \\
& 45 A^2 B^5 X^9 Y^5 + 594 A^4 B^5 X^9 Y^5 + 525 A^6 B^5 X^9 Y^5 + 45 A^3 B^6 X^9 Y^5 + 525 A^5 B^6 X^9 Y^5 + \\
& 45 A^4 B^7 X^9 Y^5 + 5 A^4 B X^{10} Y^5 + 75 A^3 B^2 X^{10} Y^5 + 5 A^5 B^2 X^{10} Y^5 + 75 A^2 B^3 X^{10} Y^5 + 80 A^4 B^3 X^{10} Y^5 + \\
& 5 A^6 B^3 X^{10} Y^5 + 5 A B^4 X^{10} Y^5 + 80 A^3 B^4 X^{10} Y^5 + 75 A^5 B^4 X^{10} Y^5 + 5 A^7 B^4 X^{10} Y^5 + 5 A^2 B^5 X^{10} Y^5 + \\
& 75 A^4 B^5 X^{10} Y^5 + 80 A^6 B^5 X^{10} Y^5 + 5 A^8 B^5 X^{10} Y^5 + 5 A^3 B^6 X^{10} Y^5 + 80 A^5 B^6 X^{10} Y^5 + \\
& 75 A^7 B^6 X^{10} Y^5 + 5 A^4 B^7 X^{10} Y^5 + 75 A^6 B^7 X^{10} Y^5 + 5 A^5 B^8 X^{10} Y^5 + A^6 X^7 Y^6 + 196 A^5 B X^7 Y^6 + \\
& 3066 A^4 B^2 X^7 Y^6 + 7294 A^3 B^3 X^7 Y^6 + 3066 A^2 B^4 X^7 Y^6 + 196 A B^5 X^7 Y^6 + B^6 X^7 Y^6 + \\
& 504 A^5 B X^8 Y^6 + 8720 A^4 B^2 X^8 Y^6 + 504 A^6 B^2 X^8 Y^6 + 20926 A^3 B^3 X^8 Y^6 + 8720 A^5 B^3 X^8 Y^6 + \\
& 8720 A^2 B^4 X^8 Y^6 + 20926 A^4 B^4 X^8 Y^6 + 504 A B^5 X^8 Y^6 + 8720 A^3 B^5 X^8 Y^6 + 504 A^2 B^6 X^8 Y^6 + \\
& 540 A^5 B X^9 Y^6 + 10314 A^4 B^2 X^9 Y^6 + 540 A^6 B^2 X^9 Y^6 + 25170 A^3 B^3 X^9 Y^6 + 12270 A^5 B^3 X^9 Y^6 + \\
& 540 A^7 B^3 X^9 Y^6 + 10314 A^2 B^4 X^9 Y^6 + 30942 A^4 B^4 X^9 Y^6 + 10314 A^6 B^4 X^9 Y^6 + 540 A B^5 X^9 Y^6 + \\
& 12270 A^3 B^5 X^9 Y^6 + 25170 A^5 B^5 X^9 Y^6 + 540 A^2 B^6 X^9 Y^6 + 10314 A^4 B^6 X^9 Y^6 + 540 A^3 B^7 X^9 Y^6 + \\
& 275 A^5 B X^{10} Y^6 + 6145 A^4 B^2 X^{10} Y^6 + 275 A^6 B^2 X^{10} Y^6 + 15490 A^3 B^3 X^{10} Y^6 + 7345 A^5 B^3 X^{10} Y^6 + \\
& 275 A^7 B^3 X^{10} Y^6 + 6145 A^2 B^4 X^{10} Y^6 + 19290 A^4 B^4 X^{10} Y^6 + 7345 A^6 B^4 X^{10} Y^6 + 275 A^8 B^4 X^{10} Y^6 + \\
& 275 A B^5 X^{10} Y^6 + 7345 A^3 B^5 X^{10} Y^6 + 19290 A^5 B^5 X^{10} Y^6 + 6145 A^7 B^5 X^{10} Y^6 + 275 A^2 B^6 X^{10} Y^6 + \\
& 7345 A^4 B^6 X^{10} Y^6 + 15490 A^6 B^6 X^{10} Y^6 + 275 A^3 B^7 X^{10} Y^6 + 6145 A^5 B^7 X^{10} Y^6 + 275 A^4 B^8 X^{10} Y^6 + \\
& 66 A^5 B X^{11} Y^6 + 1815 A^4 B^2 X^{11} Y^6 + 66 A^6 B^2 X^{11} Y^6 + 4818 A^3 B^3 X^{11} Y^6 + 2112 A^5 B^3 X^{11} Y^6 + \\
& 66 A^7 B^3 X^{11} Y^6 + 1815 A^2 B^4 X^{11} Y^6 + 5808 A^4 B^4 X^{11} Y^6 + 2079 A^6 B^4 X^{11} Y^6 + 66 A^8 B^4 X^{11} Y^6 + \\
& 66 A B^5 X^{11} Y^6 + 2112 A^3 B^5 X^{11} Y^6 + 5720 A^5 B^5 X^{11} Y^6 + 2112 A^7 B^5 X^{11} Y^6 + 66 A^9 B^5 X^{11} Y^6 + \\
& 66 A^2 B^6 X^{11} Y^6 + 2079 A^4 B^6 X^{11} Y^6 + 5808 A^6 B^6 X^{11} Y^6 + 1815 A^8 B^6 X^{11} Y^6 + 66 A^3 B^7 X^{11} Y^6 + \\
& 2112 A^5 B^7 X^{11} Y^6 + 4818 A^7 B^7 X^{11} Y^6 + 66 A^4 B^8 X^{11} Y^6 + 1815 A^6 B^8 X^{11} Y^6 + 66 A^5 B^9 X^{11} Y^6 + \\
& 6 A^5 B X^{12} Y^6 + 210 A^4 B^2 X^{12} Y^6 + 6 A^6 B^2 X^{12} Y^6 + 604 A^3 B^3 X^{12} Y^6 + 240 A^5 B^3 X^{12} Y^6 + \\
& 6 A^7 B^3 X^{12} Y^6 + 210 A^2 B^4 X^{12} Y^6 + 690 A^4 B^4 X^{12} Y^6 + 222 A^6 B^4 X^{12} Y^6 + 6 A^8 B^4 X^{12} Y^6 + \\
& 6 A B^5 X^{12} Y^6 + 240 A^3 B^5 X^{12} Y^6 + 642 A^5 B^5 X^{12} Y^6 + 222 A^7 B^5 X^{12} Y^6 + 6 A^9 B^5 X^{12} Y^6 + \\
& 6 A^2 B^6 X^{12} Y^6 + 222 A^4 B^6 X^{12} Y^6 + 642 A^6 B^6 X^{12} Y^6 + 240 A^8 B^6 X^{12} Y^6 + 6 A^{10} B^6 X^{12} Y^6 + \\
& 6 A^3 B^7 X^{12} Y^6 + 222 A^5 B^7 X^{12} Y^6 + 690 A^7 B^7 X^{12} Y^6 + 210 A^9 B^7 X^{12} Y^6 + 6 A^4 B^8 X^{12} Y^6 + \\
& 240 A^6 B^8 X^{12} Y^6 + 604 A^8 B^8 X^{12} Y^6 + 6 A^5 B^9 X^{12} Y^6 + 210 A^7 B^9 X^{12} Y^6 + 6 A^6 B^{10} X^{12} Y^6
\end{aligned}$$

$$\begin{aligned}
\text{Out[1267]} = & \left\{ 0.126428, -\frac{X}{-1+X} + \left( -\frac{A X^2}{(-1+X)^3} - \frac{B X^2}{(-1+X)^3} \right) Y + \right. \\
& \left( -\frac{6 A B X^3}{(-1+X)^5} - \frac{B^2 X^3 (1+X)}{(-1+X)^5} + A^2 \left( -\frac{2 B^2 X^4}{(-1+X)^5} - \frac{X^3 (1+X)}{(-1+X)^5} \right) \right) Y^2 + \\
& \left( -\frac{3 A^4 B^3 X^6}{(-1+X)^7} - \frac{10 A B^2 X^4 (2+X)}{(-1+X)^7} + A^2 \left( -\frac{15 B^3 X^5}{(-1+X)^7} - \frac{10 B X^4 (2+X)}{(-1+X)^7} \right) \right) -
\end{aligned}$$

$$\begin{aligned}
 & \frac{B^3 X^4 (1 + X (3 + X))}{(-1 + X)^7} + A^3 \left( -\frac{15 B^2 X^5}{(-1 + X)^7} - \frac{3 B^4 X^6}{(-1 + X)^7} - \frac{X^4 (1 + X (3 + X))}{(-1 + X)^7} \right) \Bigg) Y^3 + \\
 & \left( -\frac{4 A^6 B^4 X^8}{(-1 + X)^9} + A^5 \left( -\frac{28 B^3 X^7}{(-1 + X)^9} - \frac{20 B^5 X^8}{(-1 + X)^9} \right) - \frac{B^4 X^5 (1 + X (1 + X (5 + X)))}{(-1 + X)^9} - \right. \\
 & \quad \left. \frac{5 A B^3 X^5 (10 + 3 X (5 + X))}{(-1 + X)^9} + \right. \\
 & \quad A^4 \left( \frac{28 B^4 (-4 + X) X^7}{(-1 + X)^9} - \frac{4 B^6 X^8}{(-1 + X)^9} - \frac{21 B^2 X^6 (3 + X)}{(-1 + X)^9} - \frac{X^5 (1 + X (1 + X (5 + X)))}{(-1 + X)^9} \right) + \\
 & \quad A^3 \left( -\frac{28 B^5 X^7}{(-1 + X)^9} - \frac{5 B X^5 (10 + 3 X (5 + X))}{(-1 + X)^9} - \frac{4 B^3 X^6 (56 + X (-7 + 4 X))}{(-1 + X)^9} \right) + \\
 & \quad A^2 \left( -\frac{21 B^4 X^6 (3 + X)}{(-1 + X)^9} + \frac{2 B^2 X^5 (-80 + X (-49 + (-12 + X) X))}{(-1 + X)^9} \right) \Bigg) Y^4 + \\
 & \left( -\frac{5 A^8 B^5 X^{10}}{(-1 + X)^{11}} + A^7 \left( -\frac{45 B^4 X^9}{(-1 + X)^{11}} - \frac{75 B^6 X^{10}}{(-1 + X)^{11}} \right) + \right. \\
 & \quad A^6 \left( -\frac{75 B^7 X^{10}}{(-1 + X)^{11}} - \frac{36 B^3 X^8 (4 + X)}{(-1 + X)^{11}} + \frac{5 B^5 X^9 (-105 + 29 X)}{(-1 + X)^{11}} \right) - \\
 & \quad \frac{21 A B^4 X^6 (5 + X (15 + X (9 + X)))}{(-1 + X)^{11}} - \frac{B^5 X^6 (1 + X (10 + X (20 + X (10 + X))))}{(-1 + X)^{11}} + \\
 & \quad A^2 \left( -\frac{28 B^5 X^7 (7 + X (7 + X))}{(-1 + X)^{11}} - \frac{4 B^3 X^6 (202 + X (228 + X (93 + 2 X)))}{(-1 + X)^{11}} \right) + \\
 & \quad A^4 \left( -\frac{45 B^7 X^9}{(-1 + X)^{11}} - \frac{3 B^5 X^8 (464 + X (-157 + 33 X))}{(-1 + X)^{11}} - \frac{21 B X^6 (5 + X (15 + X (9 + X)))}{(-1 + X)^{11}} + \right. \\
 & \quad \left. \frac{B^3 X^7 (-1687 + X (-19 + X (-238 + 19 X)))}{(-1 + X)^{11}} \right) + A^3 \left( -\frac{36 B^6 X^8 (4 + X)}{(-1 + X)^{11}} - \right. \\
 & \quad \left. \frac{4 B^2 X^6 (202 + X (228 + X (93 + 2 X)))}{(-1 + X)^{11}} + \frac{B^4 X^7 (-1687 + X (-19 + X (-238 + 19 X)))}{(-1 + X)^{11}} \right) + \\
 & \quad A^5 \left( -\frac{5 B^8 X^{10}}{(-1 + X)^{11}} + \frac{5 B^6 X^9 (-105 + 29 X)}{(-1 + X)^{11}} - \frac{28 B^2 X^7 (7 + X (7 + X))}{(-1 + X)^{11}} - \right. \\
 & \quad \left. \frac{3 B^4 X^8 (464 + X (-157 + 33 X))}{(-1 + X)^{11}} - \frac{X^6 (1 + X (10 + X (20 + X (10 + X))))}{(-1 + X)^{11}} \right) \Bigg) Y^5 + \\
 & \left( -\frac{6 A^{10} B^6 X^{12}}{(-1 + X)^{13}} + A^9 \left( -\frac{66 B^5 X^{11}}{(-1 + X)^{13}} - \frac{210 B^7 X^{12}}{(-1 + X)^{13}} \right) + \right. \\
 & \quad A^8 \left( -\frac{604 B^8 X^{12}}{(-1 + X)^{13}} - \frac{55 B^4 X^{10} (5 + X)}{(-1 + X)^{13}} + \frac{15 B^6 X^{11} (-121 + 31 X)}{(-1 + X)^{13}} \right) + \\
 & \quad A^7 \left( -\frac{210 B^9 X^{12}}{(-1 + X)^{13}} + \frac{6 B^7 X^{11} (-803 + 290 X)}{(-1 + X)^{13}} + \frac{B^5 X^{10} (-6145 + (2313 - 350 X) X)}{(-1 + X)^{13}} - \right. \\
 & \quad \left. \frac{45 B^3 X^9 (12 + X (9 + X))}{(-1 + X)^{13}} \right) - \frac{B^6 X^7 (1 + X (1 + X (14 + X (36 + X (14 + X))))}{(-1 + X)^{13}} -
 \end{aligned}$$

$$\begin{aligned}
& \frac{28 A B^5 X^7 (7 + X (35 + X (42 + X (14 + X))))}{(-1 + X)^{13}} + A^6 \left( -\frac{6 B^{10} X^{12}}{(-1 + X)^{13}} + \frac{15 B^8 X^{11} (-121 + 31 X)}{(-1 + X)^{13}} - \right. \\
& \frac{2 B^6 X^{10} (7745 - 4380 X + 968 X^2)}{(-1 + X)^{13}} + \frac{2 B^4 X^9 (-5157 + X (1211 - 558 X + 40 X^2))}{(-1 + X)^{13}} - \\
& \left. \frac{36 B^2 X^8 (14 + X (28 + X (12 + X)))}{(-1 + X)^{13}} - \frac{X^7 (1 + X) (1 + X (14 + X (36 + X (14 + X))))}{(-1 + X)^{13}} \right) + \\
& A^5 \left( -\frac{66 B^9 X^{11}}{(-1 + X)^{13}} + \frac{B^7 X^{10} (-6145 + (2313 - 350 X) X)}{(-1 + X)^{13}} - \right. \\
& \frac{B^3 X^8 (8720 + X (3490 + X (1985 + 37 X)))}{(-1 + X)^{13}} + \\
& \frac{2 B^5 X^9 (-12585 + X (6585 + X (-3091 + 496 X)))}{(-1 + X)^{13}} - \\
& \left. \frac{28 B X^7 (7 + X (35 + X (42 + X (14 + X))))}{(-1 + X)^{13}} \right) + \\
& A^3 \left( -\frac{45 B^7 X^9 (12 + X (9 + X))}{(-1 + X)^{13}} - \frac{B^5 X^8 (8720 + X (3490 + X (1985 + 37 X)))}{(-1 + X)^{13}} + \right. \\
& \left. \frac{1}{(-1 + X)^{13}} 2 B^3 X^7 (-3647 + X (-4536 + X (-3133 + 2 (-10 + X) X (9 + 4 X)))) \right) + \\
& A^4 \left( -\frac{55 B^8 X^{10} (5 + X)}{(-1 + X)^{13}} + \frac{2 B^6 X^9 (-5157 + X (1211 - 558 X + 40 X^2))}{(-1 + X)^{13}} - \right. \\
& \frac{1}{(-1 + X)^{13}} 2 B^4 X^8 (10463 + X (-443 + 3 X (1167 - 240 X + 38 X^2))) - \\
& \left. \frac{2 B^2 X^7 (1533 + X (3071 + X (1969 + X (352 + 5 X))))}{(-1 + X)^{13}} \right) + \\
& A^2 \left( -\frac{36 B^6 X^8 (14 + X (28 + X (12 + X)))}{(-1 + X)^{13}} - \right. \\
& \left. \frac{2 B^4 X^7 (1533 + X (3071 + X (1969 + X (352 + 5 X))))}{(-1 + X)^{13}} \right) \Bigg\} Y^6 \Bigg\} \\
\text{Out[1268]= } & \left\{ 0.115034, W + \left( -\frac{A W^2 (1 + W)}{-1 + W} - \frac{B W^2 (1 + W)}{-1 + W} \right) Y + \right. \\
& \left( \frac{B^2 W^3 (-1 - 3 W + 2 W^3)}{(-1 + W)^3} - \frac{2 A B W^3 (1 + W) (3 + W (-1 + (-2 + W) W))}{(-1 + W)^3} + \right. \\
& \left. A^2 \left( -\frac{2 B^2 W^4 (1 + W)}{-1 + W} + \frac{W^3 (-1 - 3 W + 2 W^3)}{(-1 + W)^3} \right) \right) Y^2 + \\
& \left( -\frac{3 A^4 B^3 W^6 (1 + W)}{-1 + W} - \frac{B^3 W^4 (1 + W) (1 + W (6 + 5 (-2 + W) W^2))}{(-1 + W)^5} + A^3 \left( -\frac{3 B^4 W^6 (1 + W)}{-1 + W} - \right. \right. \\
& \left. \frac{W^4 (1 + W) (1 + W (6 + 5 (-2 + W) W^2))}{(-1 + W)^5} - \frac{B^2 W^5 (1 + W) (15 + W (-3 + W (-11 + 3 W)))}{(-1 + W)^3} \right) \Bigg) -
\end{aligned}$$



$$\begin{aligned}
 & \frac{1}{(-1+W)^5} A B^2 W^4 (1+W) (20+W (5+W (-43+W (16+(-2+W) W (-11+3 W)))) + \\
 & A^2 \left( -\frac{B^3 W^5 (1+W) (15+W (-3+W (-11+3 W)))}{(-1+W)^3} - \frac{1}{(-1+W)^5} \right. \\
 & \left. B W^4 (1+W) (20+W (5+W (-43+W (16+(-2+W) W (-11+3 W)))) \right) \Bigg) Y^3 + \\
 & \left( -\frac{4 A^6 B^4 W^8 (1+W)}{-1+W} + A^5 \left( -\frac{20 B^5 W^8 (1+W)}{-1+W} - \frac{2 B^3 W^7 (1+W) (14+W (-2+W (-11+2 W)))}{(-1+W)^3} \right) \right) + \\
 & \frac{1}{(-1+W)^7} B^4 W^5 (1+W) (-1+W (-12+W (-19+W (34+7 W (3+2 (-3+W) W)))) + \\
 & A^4 \left( -\frac{4 B^6 W^8 (1+W)}{-1+W} - \frac{4 B^4 W^7 (1+W) (28+W (-19+5 (-2+W) W))}{(-1+W)^3} + \frac{1}{(-1+W)^7} \right. \\
 & \left. W^5 (1+W) (-1+W (-12+W (-19+W (34+7 W (3+2 (-3+W) W)))) - \frac{1}{(-1+W)^5} \right. \\
 & \left. B^2 W^6 (1+W) (63+W (14+W (-122+W (24+W (59-30 W+4 W^2)))) \right) \Bigg) + \\
 & A^2 \left( -\frac{1}{(-1+W)^5} B^4 W^6 (1+W) (63+W (14+W (-122+W (24+W (59-30 W+4 W^2)))) - \right. \\
 & \left. \frac{1}{(-1+W)^7} 2 B^2 W^5 (1+W) (80+W (-14+ \right. \\
 & \left. W (-196+W (100+(-2+W) W (-116+W (63+2 W (19+5 (-4+W) W)))) \right) \Bigg) - \\
 & \frac{1}{(-1+W)^7} A B^3 W^5 (1+W) (50+W (87+W (-200+W (-79+W (324+ \\
 & W (-127+W (-124+W (123-38 W+4 W^2)))))) + \\
 & A^3 \left( -\frac{2 B^5 W^7 (1+W) (14+W (-2+W (-11+2 W)))}{(-1+W)^3} - \frac{1}{(-1+W)^5} 2 B^3 W^6 (1+W) \right. \\
 & \left. (112+W (-91+W (-90+W (74+W (44+W (-47+10 W)))) - \right. \\
 & \left. \frac{1}{(-1+W)^7} B W^5 (1+W) (50+W (87+W (-200+ \right. \\
 & \left. W (-79+W (324+W (-127+W (-124+W (123-38 W+4 W^2)))) \right) \Bigg) \Bigg) Y^4 + \\
 & \left( -\frac{5 A^8 B^5 W^{10} (1+W)}{-1+W} + A^7 \left( -\frac{75 B^6 W^{10} (1+W)}{-1+W} - \frac{B^4 W^9 (1+W) (45+W (-5+W (-37+5 W)))}{(-1+W)^3} \right) \right) + \\
 & A^6 \left( -\frac{75 B^7 W^{10} (1+W)}{-1+W} - \frac{5 B^5 (-3+W) W^9 (1+W) (-35+W (13+16 W))}{(-1+W)^3} - \frac{1}{(-1+W)^5} B^3 W^8 \right. \\
 & \left. (1+W) (144+W (27+W (-273+W (32+W (130+W (-47+5 W)))) \right) \Bigg) - \frac{1}{(-1+W)^9} \\
 & B^5 W^6 (1+W) (21+W (96+W (56+W (-237+7 W (-15+2 W (20+3 (-3+W) W^2)))) + \\
 & A^5 \left( -\frac{5 B^8 W^{10} (1+W)}{-1+W} - \right.
 \end{aligned}$$

$$\begin{aligned}
& \frac{5 B^6 (-3 + W) W^9 (1 + W) (-35 + W (13 + 16 W))}{(-1 + W)^3} - \frac{1}{(-1 + W)^5} B^4 W^8 (1 + W) \\
& \left( (1392 + W (-1536 + W (-691 + W (998 + W (194 - 354 W + 75 W^2)))) \right) - \frac{1}{(-1 + W)^9} \\
& W^6 (1 + W (21 + W (96 + W (56 + W (-237 + 7 W (-15 + 2 W (20 + 3 (-3 + W) W^2)))))) - \\
& \frac{1}{(-1 + W)^7} B^2 W^7 (1 + W) (196 + W (248 + W (-654 + W (-265 + W (863 + \\
& W (-201 + (-4 + W) W (81 + W (-37 + 5 W)))))) \left) - \frac{1}{(-1 + W)^9} A B^4 \right. \\
& W^6 (1 + W) (105 + W (434 + W (-396 + W (-1296 + W (1664 + W (817 + W (-2372 + W (991 + \\
& W (676 + W (-839 + W (348 + W (-67 + 5 W)))))))))) + \\
& A^4 \left( - \frac{B^7 W^9 (1 + W) (45 + W (-5 + W (-37 + 5 W)))}{(-1 + W)^3} - \frac{1}{(-1 + W)^5} B^5 W^8 (1 + W) \right. \\
& \left( (1392 + W (-1536 + W (-691 + W (998 + W (194 - 354 W + 75 W^2)))) \right) - \\
& \frac{1}{(-1 + W)^7} B^3 W^7 (1 + W) (1687 + W (-1586 + W (-2142 + W (2176 + \\
& W (1977 + 2 W (-1305 + W (-26 + W (562 + W (-267 + 40 W)))))) - \\
& \frac{1}{(-1 + W)^9} B W^6 (1 + W) (105 + W (434 + W (-396 + W (-1296 + W (1664 + \\
& W (817 + W (-2372 + W (991 + W (676 + W (-839 + \\
& W (348 + W (-67 + 5 W)))))) \left) + A^3 \right. \\
& \left( - \frac{1}{(-1 + W)^5} B^6 W^8 (1 + W) (144 + W (27 + W (-273 + W (32 + W (130 + W (-47 + 5 W)))) - \right. \\
& \frac{1}{(-1 + W)^7} B^4 W^7 (1 + W) (1687 + W (-1586 + W (-2142 + W (2176 + \\
& W (1977 + 2 W (-1305 + W (-26 + W (562 + W (-267 + 40 W)))))) - \\
& \frac{1}{(-1 + W)^9} B^2 W^6 (1 + W) (808 + W (137 + W (-2944 + W (806 + W (5821 + \\
& W (-5191 + W (-3236 + W (6665 + W (-2180 + W (-1850 + \\
& W (1844 + 15 W (-41 + 5 W)))))) \left) + \right. \\
& A^2 \left( - \frac{1}{(-1 + W)^7} B^5 W^7 (1 + W) (196 + W (248 + W (-654 + W (-265 + W (863 + \\
& W (-201 + (-4 + W) W (81 + W (-37 + 5 W)))))) - \frac{1}{(-1 + W)^9} \right. \\
& B^3 W^6 (1 + W) (808 + W (137 + W (-2944 + W (806 + W (5821 + W (-5191 + W (-3236 + \\
& W (6665 + W (-2180 + W (-1850 + W (1844 + 15 W (-41 + \\
& 5 W)))))) \left) \right) Y^5 + \left( - \frac{6 A^{10} B^6 W^{12} (1 + W)}{-1 + W} + \right. \\
& A^9 \left( - \frac{210 B^7 W^{12} (1 + W)}{-1 + W} - \frac{2 B^5 W^{11} (1 + W) (33 + W (-3 + W (-28 + 3 W)))}{(-1 + W)^3} \right) + \\
& A^8
\end{aligned}$$

$$\begin{aligned}
 & \left( -\frac{604 B^8 W^{12} (1+W)}{-1+W} - \frac{5 B^6 W^{11} (1+W) (363+2 W (-117-70 W+24 W^2))}{(-1+W)^3} - \frac{1}{(-1+W)^5} \right. \\
 & \quad \left. B^4 W^{10} (1+W) (275+W (44+W (-520+W (40+W (247-68 W+6 W^2)))) \right) + \\
 & \quad \frac{1}{(-1+W)^{11}} B^6 W^7 (1+W) (-1+W (-30+W (-200+W (-230+ \\
 & \quad \quad W (705+2 W (274+3 W (-236+W (20+11 W (15+2 (-5+W) W)))))) + \\
 A^7 & \left( -\frac{210 B^9 W^{12} (1+W)}{-1+W} - \frac{2 B^7 W^{11} (1+W) (2409+5 W (-417+W (-94+69 W)))}{(-1+W)^3} - \right. \\
 & \quad \frac{1}{(-1+W)^5} B^5 W^{10} (1+W) \\
 & \quad (6145+W (-6738+W (-3436+W (4634+W (609+2 W (-598+111 W)))))) - \\
 & \quad \frac{1}{(-1+W)^7} B^3 W^9 (1+W) (540+W (535+W (-1702+ \\
 & \quad \quad W (-633+W (2016+W (-273+W (-738+W (389-80 W+6 W^2)))))) \right) + \\
 A^6 & \left( -\frac{6 B^{10} W^{12} (1+W)}{-1+W} - \frac{5 B^8 W^{11} (1+W) (363+2 W (-117-70 W+24 W^2))}{(-1+W)^3} - \right. \\
 & \quad \frac{1}{(-1+W)^5} 2 B^6 W^{10} (1+W) \\
 & \quad (7745+W (-11664+W (831+W (4462+W (-253+3 W (-406+107 W)))))) - \\
 & \quad \frac{1}{(-1+W)^7} B^4 W^9 (1+W) (10314+W (-12189+W (-10646+W (15795+W \\
 & \quad \quad (5504+W (-11401+W (738+W (3685+6 W (-277+37 W)))))) \right) + \\
 & \quad \frac{1}{(-1+W)^{11}} W^7 (1+W) (-1+W (-30+W (-200+W (-230+W (705+2 W \\
 & \quad \quad (274+3 W (-236+W (20+11 W (15+2 (-5+W) W)))))) - \\
 & \quad \frac{1}{(-1+W)^9} B^2 W^8 (1+W) (504+W (1476+W (-1847+W (-4020+W (4986+W (2656+ \\
 & \quad \quad W (-5904+W (1656+W (1760+W (-1596+W (555-92 W+ \\
 & \quad \quad \quad 6 W^2)))))) \right) - \frac{1}{(-1+W)^{11}} A B^5 W^7 (1+W) \\
 & \quad (196+W (1456+W (580+W (-6775+W (1508+W (13799+W (-12672+W (-7002+ \\
 & \quad \quad \quad W (16890+W (-7624+W (-3460+W (5507+W (-2798+ \\
 & \quad \quad \quad W (745+2 W (-52+3 W)))))) \right) + \\
 A^4 & \left( -\frac{1}{(-1+W)^5} B^8 W^{10} (1+W) (275+W (44+W (-520+W (40+W (247-68 W+6 W^2)))) \right) - \\
 & \quad \frac{1}{(-1+W)^7} B^6 W^9 (1+W) (10314+W (-12189+W (-10646+W (15795+W \\
 & \quad \quad (5504+W (-11401+W (738+W (3685+6 W (-277+37 W)))))) - \\
 & \quad \frac{1}{(-1+W)^9} 2 B^4 W^8 (1+W) (10463+W (-16357+W (-6417+W (16534+ \\
 & \quad \quad W (18775+W (-36510+W (856+W (27472+W (-14439+W (-5005+ \\
 & \quad \quad \quad W (7397+3 W (-898+115 W)))))) \right) -
 \end{aligned}$$

$$\begin{aligned} & \frac{1}{(-1+W)^{11}} B^2 W^7 (1+W) (3066 + W (3564 + W (-16368 + W (-5995 + W \\ & \quad (50017 + W (-22911 + W (-66244 + W (79064 + W (10085 + \\ & \quad \quad W (-70552 + W (41600 + W (6995 + W (-19626 + \\ & \quad \quad \quad 5W(2009 - 464W + 42W^2))))))))) + \\ A^2 & \left( -\frac{1}{(-1+W)^9} B^6 W^8 (1+W) (504 + W (1476 + W (-1847 + W (-4020 + W (4986 + \right. \\ & \quad \quad W (2656 + W (-5904 + W (1656 + W (1760 + \\ & \quad \quad \quad W (-1596 + W (555 - 92W + 6W^2))))))))) - \\ & \frac{1}{(-1+W)^{11}} B^4 W^7 (1+W) (3066 + W (3564 + W (-16368 + W (-5995 + W \\ & \quad (50017 + W (-22911 + W (-66244 + W (79064 + W (10085 + \\ & \quad \quad W (-70552 + W (41600 + W (6995 + W (-19626 + \\ & \quad \quad \quad 5W(2009 - 464W + 42W^2))))))))) + \\ A^3 & \left( -\frac{1}{(-1+W)^7} B^7 W^9 (1+W) (540 + W (535 + W (-1702 + W (-633 + W (2016 + \right. \\ & \quad \quad W (-273 + W (-738 + W (389 - 80W + 6W^2)))))) ) - \frac{1}{(-1+W)^9} \\ & B^5 W^8 (1+W) (8720 + W (-5290 + W (-21595 + W (15564 + W (29676 + \\ & \quad \quad W (-31780 + W (-14538 + W (31944 + W (-8820 + W (-8882 + \\ & \quad \quad \quad W (7549 + 4W (-557 + 60W))))))))) - \\ & \frac{1}{(-1+W)^{11}} 2B^3 W^7 (1+W) (3647 + W (-1391 + W (-12819 + W (5690 + \\ & \quad \quad W (37469 + W (-42563 + W (-29682 + W (76604 + W (-22705 + \\ & \quad \quad \quad W (-47879 + W (46309 + W (-5132 + W (-14695 + \\ & \quad \quad \quad \quad W (10065 - 2800W + 302W^2))))))))) + \\ A^5 & \left( -\frac{2B^9 W^{11}(1+W)(33 + W(-3 + W(-28 + 3W)))}{(-1+W)^3} - \frac{1}{(-1+W)^5} B^7 W^{10}(1+W) \right. \\ & \quad (6145 + W (-6738 + W (-3436 + W (4634 + W (609 + 2W (-598 + 111W)))))) - \\ & \frac{1}{(-1+W)^7} 6B^5 W^9 (1+W) (4195 + W (-7605 + W (1062 + W (4264 + \\ & \quad \quad W (380 + W (-3722 + W (1086 + W (964 + W (-631 + 107W)))))) ) - \\ & \frac{1}{(-1+W)^9} B^3 W^8 (1+W) (8720 + W (-5290 + W (-21595 + W (15564 + W (29676 + \\ & \quad \quad W (-31780 + W (-14538 + W (31944 + W (-8820 + W (-8882 + \\ & \quad \quad \quad W (7549 + 4W (-557 + 60W))))))))) - \\ & \frac{1}{(-1+W)^{11}} B W^7 (1+W) (196 + W (1456 + W (580 + W (-6775 + W (1508 + \\ & \quad \quad W (13799 + W (-12672 + W (-7002 + W (16890 + \\ & \quad \quad \quad W (-7624 + W (-3460 + W (5507 + W (-2798 + \\ & \quad \quad \quad \quad W (745 + 2W (-52 + 3W))))))))) \Bigg) Y^6 \end{aligned}$$

```

Out[1269]= 
$$-\frac{1}{(-1+W)^{11}}$$


$$2 W^7 (1+W) (6910+W (23346+W (-64513+W (-90740+W (326204+W (-38334+W$$


$$(-639407+W (606796+W (278270+W (-793738+$$


$$W (399105+W (155508+W (-279128+W$$


$$(141910+W (-34161+3316 W))))))))))$$


Out[1270]= 
$$13820 + 46692 W - 129026 W^2 - 181480 W^3 + 652408 W^4 -$$


$$76668 W^5 - 1278814 W^6 + 1213592 W^7 + 556540 W^8 - 1587476 W^9 +$$


$$798210 W^{10} + 311016 W^{11} - 558256 W^{12} + 283820 W^{13} - 68322 W^{14} + 6632 W^{15}$$


```
